# Supplementary material for: MetaShift: A Dataset of Datasets for Evaluating Contextual Distribution Shifts and Training Conflicts
Source: arXiv:2202.06523 source file (2022-02-14)
Supplement: Supplementary file 1 [file checklist.tex]

%%%%%%%%%%%%%%%%%%%%%%%%%%%%%%%%%%%%%%%%%%%%%%%%%%%%%%%%%%%%
\section*{Checklist}

%%% BEGIN INSTRUCTIONS %%%
% The checklist follows the references.  Please
% read the checklist guidelines carefully for information on how to answer these
% questions.  For each question, change the default \answerTODO{} to \answerYes{},
% \answerNo{}, or \answerNA{}.  You are strongly encouraged to include a {\bf
% justification to your answer}, either by referencing the appropriate section of
% your paper or providing a brief inline description.  For example:
% \begin{itemize}
%   \item Did you include the license to the code and datasets? \answerYes{See Section~\ref{gen_inst}.}
%   \item Did you include the license to the code and datasets? \answerNo{The code and the data are proprietary.}
%   \item Did you include the license to the code and datasets? \answerNA{}
% \end{itemize}
% Please do not modify the questions and only use the provided macros for your
% answers.  Note that the Checklist section does not count towards the page
% limit.  In your paper, please delete this instructions block and only keep the
% Checklist section heading above along with the questions/answers below.
%%% END INSTRUCTIONS %%%

\begin{enumerate}

\item For all authors...
\begin{enumerate}
  \item Do the main claims made in the abstract and introduction accurately reflect the paper's contributions and scope?
    \answerYes{} % \answerTODO{}
  \item Did you describe the limitations of your work?
    \answerYes{}  % \answerTODO{}
  \item Did you discuss any potential negative societal impacts of your work?
    \answerYes{} % \answerTODO{}
  \item Have you read the ethics review guidelines and ensured that your paper conforms to them?
    \answerYes{} % \answerTODO{}
\end{enumerate}

\item If you are including theoretical results...
\begin{enumerate}
  \item Did you state the full set of assumptions of all theoretical results?
    \answerNA{} % \answerTODO{}
	\item Did you include complete proofs of all theoretical results?
     \answerNA{} % \answerTODO{}
\end{enumerate}

\item If you ran experiments...
\begin{enumerate}
  \item Did you include the code, data, and instructions needed to reproduce the main experimental results (either in the supplemental material or as a URL)?
    \answerYes{Please refer to the supplemental material.} % \answerTODO{}
  \item Did you specify all the training details (e.g., data splits, hyperparameters, how they were chosen)?
     \answerYes{We use the implementation and hyper-parameters from Domainbed~\citep{gulrajani2020search} for empirical risk minimization (ERM) and all domain generalization baselines. } % \answerTODO{}
	\item Did you report error bars (e.g., with respect to the random seed after running experiments multiple times)?
    \answerYes{We repeat our experiments on the same test set multiple times, although with different training data. Due to the large number of experiments and the time constraint, we did not have error bars in the table. }
	\item Did you include the total amount of compute and the type of resources used (e.g., type of GPUs, internal cluster, or cloud provider)?
    \answerYes{The experiments are conducted on an Amazon EC2 P3.8 instance with 4 NVIDIA V100 Tensor Core GPUs. The training takes less than an hour to finish. } % \answerTODO{}
\end{enumerate}

\item If you are using existing assets (e.g., code, data, models) or curating/releasing new assets...
\begin{enumerate}
  \item If your work uses existing assets, did you cite the creators?
    \answerYes{We have cited Visual Genome~\citep{VisualGenome} and Domainbed~\citep{gulrajani2020search} } % \answerTODO{}
  \item Did you mention the license of the assets?
    \answerYes{Visual Genome~\citep{VisualGenome} is licensed under a Creative Commons Attribution 4.0 International License. Our Meta-Dataset and the code for generating it would use the same licence. Domainbed is licensed under an MIT License. } % \answerTODO{}
  \item Did you include any new assets either in the supplemental material or as a URL?
    \answerYes{} % \answerTODO{}
  \item Did you discuss whether and how consent was obtained from people whose data you're using/curating?
    \answerYes{} % \answerTODO{}
  \item Did you discuss whether the data you are using/curating contains personally identifiable information or offensive content?
    \answerYes{To the best of our knowledge, Visual Genome has removed personally identifiable information or offensive content during data-set creation, so our Meta-Dataset does not contain these kinds of content. } % \answerTODO{}
\end{enumerate}

\item If you used crowdsourcing or conducted research with human subjects...
\begin{enumerate}
  \item Did you include the full text of instructions given to participants and screenshots, if applicable?
    \answerNA{} % \answerTODO{}
  \item Did you describe any potential participant risks, with links to Institutional Review Board (IRB) approvals, if applicable?
    \answerNA{} % \answerTODO{}
  \item Did you include the estimated hourly wage paid to participants and the total amount spent on participant compensation?
    \answerNA{} % \answerTODO{}
\end{enumerate}

\end{enumerate}

%%%%%%%%%%%%%%%%%%%%%%%%%%%%%%%%%%%%%%%%%%%%%%%%%%%%%%%%%%%%
